# Supplementary material for: HELP: Hardware-Adaptive Efficient Latency Prediction for NAS via Meta-Learning
Source: arXiv:2106.08630 source file (2021-12-02)
Supplement: Supplementary file 1 [file suppl_ofa.tex]

\FloatBarrier
\begin{table}[h]
    \begin{center}
    \caption{\small Comparison of NAS results on ImageNet using unseen platform device, Jetson AGX Xavier. By combining HELP with rapid NAS method such as OFA, we can obtain competitive latency-constrained architecture against architectures from other state-of-the-art NAS methods, reducing total NAS cost significantly.
    } 
    %\vspace{-0.1in}
    \label{tbl:suppl_ofa}
    \resizebox{\linewidth}{!}{
    
            \begin{tabular}{c|l|ccc|cc|cc}
             \toprule
             \centering
            %   \multicolumn{1}{c}{\multirow{2}{*}{Device}} & \multicolumn{1}{c|}{\multirow{2}{*}{Model}}  & MACs & Latency & Accuracy & \multicolumn{2}{c|}{Latency Model} & Total NAS Cost & Speed Up\\
              \multirow{2}{*}{Device} & \multicolumn{1}{c|}{\multirow{2}{*}{Model}}  & MACs & Latency & Accuracy & \multicolumn{2}{c|}{Latency Model} & Total NAS Cost & Speed Up\\
              & &   (M)  & (ms) & (\%) &Sample & Building Time  & (Wall Clock)&  \\
             \midrule
             \midrule

             &MobileNetV3-Large~\citep{howard2019searching}            
              & 219M   & 70.8 & 75.2   & -    & -    & - & -\\
             % \cdashline{2-10}\noalign{\vskip 0.75ex}
            % & Efficientnet B0               
            %& -     & -   & -    & 390M    & 44.4 & 77.1    \\
             Unseen Platform
            &MnasNet-A1~\citep{tan2019mnasnet}          
              & 312M  & 71.6 & 75.2  & 8k     & 24.9h     & 40,024.9h & 1.0$\times$\\

            Jetson AGX Xavier
            &ProxylessNAS-GPU~\citep{cai2018proxylessnas}          
              &  465M     & 82.6 & 75.1    & 5k    & 15.6h   & 515.6h &  78$\times$\\
            (Batch 16)
            & OFA+Layer-wise Pred.~\cite{cai2020once}     
               & 349M    & 69.2     & 75.8  &27k   & 84h & 84h  & 476$\times$\\
            \cdashline{2-9}\noalign{\vskip 0.75ex}
           
            & OFA + HELP (65ms)        
             & 243M      & 67.4    & 75.9  & \multirow{2}{*}{\textbf{10}}      & \multirow{2}{*}{\textbf{112s}}   &\multirow{2}{*}{\textbf{0.03h (112s)}} & \multirow{2}{*}{\textbf{1.3M$\times$}}\\ 
            & OFA + HELP (70ms)       
             & 279M      & 76.4    & 76.7   &       &   && \\

             \bottomrule
             \end{tabular}
            
            }
            
        \end{center}
    \vspace{-0.2in}
\end{table}% \begin{table}[t]
\FloatBarrier
