# Supplementary material for: HELP: Hardware-Adaptive Efficient Latency Prediction for NAS via Meta-Learning
Source: arXiv:2106.08630 source file (2021-12-02)
Supplement: Supplementary file 2 [file suppl_plotform_corr.tex]

\begin{table}[H]
    \begin{center}
    \caption{\small 
    } 
    %\vspace{-0.1in}
    \label{tbl:platform_corr}
    \resizebox{\linewidth}{!}{
    
            \begin{tabular}{l|cccccc}
             \toprule
             \centering
                    & GPU   & CPU   & Mobile    & Raspi4    & FPGA  & ASIC
            GPU     & 1     & 0.758 & 0.803     & 0.739     & 0.887 & 0.906
            CPU     & 0.758 & 1     & 0.892     & 0.844     & 0.943 & 0.586
            Mobile  & 0.803 & 0.892 & 1         & 0.808     & 0.924 & 0.624
            Raspi4
            FPGA
            ASIC

             \bottomrule
             \end{tabular}
            
            }
            
        \end{center}
    \vspace{-0.2in}
\end{table}% \begin{table}[t]
