# Supplementary material for: HELP: Hardware-Adaptive Efficient Latency Prediction for NAS via Meta-Learning
Source: arXiv:2106.08630 source file (2021-12-02)
Supplement: Supplementary file 3 [file 6_appendix.tex]

%%%%%%%%%%%%%%%%%%%%%%%%%%%%%%%%%%%%%%%%%%%%%%%%%%%%%%%%%%%%
